# Supplementary material for: Design Considerations for 3RRR Parallel Robots with Lightweight, Approximate Static-Balancing
Source: arXiv:2306.13156 source file (2023-06-22)
Supplement: Supplementary file 1 [file Appendices.tex]

% if have a single appendix:
%\appendix[Proof of the Zonklar Equations]
% or
%\appendix  % for no appendix heading
% do not use \section anymore after \appendix, only \section*
% is possibly needed

% use appendices with more than one appendix
% then use \section to start each appendix
% you must declare a \section before using any
% \subsection or using \label (\appendices by itself
% starts a section numbered zero.)
%

\appendix{

\begin{algorithm}[htbp] \nonumber
 \caption{Nonlinear LS Minimization}
 \label{algo:cal_1:LS}
 \begin{algorithmic}[1]
 \footnotesize
 \Require $TargetPoses(q,\Phi,\Psi)$ \Comment {Data set for minimization process}

 \State \textbf{START} Initialize: $\mb{\vec{x}}$,\hspace{2mm} $M_i \gets 100$ \Comment {Minimization parameters vector}

 \While{$M>\epsilon_{\tau} \hspace{2mm}and \hspace{2mm}iter_{i}<iter_{max}$}

     \State $\vec{\bs{\Gamma}}(\vec{x}) = \left[\bs{\Gamma}_{11}; \bs{\Gamma}_{21};...;\bs{\Gamma}_{3N}\right]$, \hspace{2mm}
          \hspace{2mm} \hspace{4mm} \Comment {Aggregated torque vector}  \Comment {N number of Target Poses}

     \State $\bigtriangleup\bs{\Gamma} = \frac{\partial\bs{\Gamma}}{\partial\vec{x}}\bigtriangleup\vec{x}$,\hspace{2mm} $\frac{\partial\bs{\Gamma}}{\partial\vec{x}} = \bs{J}_A$, \hspace{2mm} \\
     \State $\bs{J}_A = \begin{bmatrix}\frac{\partial\bs{\Gamma}_1}{\partial\vec{x}} \\ \frac{\partial\bs{\Gamma}_2}{\partial\vec{x}} \\ \vdots \\ \frac{\partial\bs{\Gamma}_{3N}}{\partial\vec{x}}\end{bmatrix}$ \Comment {Gradient of cost function}

     \State Update $\mb{\vec{x}}_{i+1}$:
     \begin{align}
       &\mb{\vec{x}}_{i+1} = \mb{\vec{x}}_i - \eta \mb{J}_A^{\boldsymbol{+}}\vec{\Gamma} \\
           %\label{eqn:algo:NLS_update_k}
       &M_i = \frac{\vec{\bs{\Gamma}}^T\vec{\bs{\Gamma}}}{2N}
          %\label{eqn:algo:J_M_plus}
    \end{align} \Comment {$\eta$ step-size matrix}
 \EndWhile
\State $\mb{\vec{x}}^{*} \gets \mb{\vec{x}}_i$
 \Ensure ${\mb{\vec{x}}^{*}}$
\end{algorithmic}
\end{algorithm} }
